# Supplementary material for: Breakdown of Ergodicity and Self-Averaging in Polar Flocks with Quenched Disorder
Source: arXiv:2010.02356 ancillary file (2021-01-12)
Supplement: Supplementary file 1 [file quenched-prl-SI.pdf]

# Supplementary Information for “Breakdown of Ergodicity and Self-Averaging in Polar Flocks with Quenched Disorder”

Yu Duan,<sup>1,2</sup> Benoît Mahault,<sup>3</sup> Yu-qiang Ma,<sup>1,2</sup> Xia-qing Shi,<sup>2</sup> and Hugues Chaté<sup>4,5</sup>

<sup>1</sup>National Laboratory of Solid State Microstructures and Department of Physics, Nanjing University, Nanjing 210093, China

<sup>2</sup>Center for Soft Condensed Matter Physics and Interdisciplinary Research, Soochow University, Suzhou 215006, China

<sup>3</sup>Max Planck Institute for Dynamics and Self-Organization (MPIDS), 37077 Göttingen, Germany

<sup>4</sup>Service de Physique de l’Etat Condensé, CEA, CNRS Université Paris-Saclay, CEA-Saclay, 91191 Gif-sur-Yvette, France

<sup>5</sup>Computational Science Research Center, Beijing 100193, China

Here we give details about the numerical protocols that have led to the data presented in the main text.

## Preparation of samples

To build a realization of quenched disorder for our models, one must draw random numbers to be assigned to each unit box  $n$ . In the RS case, these are random angles  $\alpha_n$  drawn from a zero-mean uniform distribution of width  $2\pi\varepsilon$ . At finite size  $L$ ,  $\langle\alpha_n\rangle_n$ , the average of these angles is not strictly zero. We have observed that this leads, at large-enough size, and in the homogeneous ordered phase, to a slow but steady rotation in time of the global angle  $\theta_m$ . On the other hand, when  $\langle\alpha_n\rangle_n = 0$ , no rotation is observed. (Note that in the RC case, no such steady global rotation occurs.)

This phenomenon is interesting per se, since it signals that even a minute chirality can induce global rotation in the polar liquid, but is a problem for what concerns the present study. All the samples used here have thus been constructed making sure that  $\langle\alpha_n\rangle_n = 0$ . In practice, we generate  $L^2$  numbers regularly spaced between  $-\pi\varepsilon$  and  $\pi\varepsilon$ , and then assign them randomly to the  $L^2$  unit boxes paving the spatial domain.

## Phase diagrams

The stylized phase diagrams presented in Fig. 1 of the main text have been determined from a single realization of disorder. This sample was checked to be rather ‘typical’ in the sense that it yields values of  $\langle m \rangle_t$ , the time-average of  $m$ , located ‘in the middle’ of the distribution over samples  $\text{PDF}(\langle m \rangle_t)$ , at the (few) parameter values at which this was calculated.

Only the two planes of the 3D parameter space shown in Fig. 1 of the main text have been covered thoroughly, with only partial exploration of some other planes. At each set of parameters considered,  $\langle m \rangle_t$  was calculated, taking care of excluding transients, and averaging over typically  $1\text{E}6$  timesteps. This yielded the maps  $\langle m \rangle_t(\rho_0, \varepsilon)$ ,  $\langle m \rangle_t(\rho_0, \eta)$ , and  $\langle m \rangle_t(\eta, \varepsilon)$  shown in Fig. S1. The lines separating the disordered phase from the ordered ones (either homogeneous or band-based) were determined by the contour lines at  $\langle m \rangle_t = 0.25$ , a value typical of the ‘middle ground’ between disorder and order.

The limits of the band phase were delimited visually,

by inspection of snapshots and movies constructed from the runs described above. At parameter values for which the diagnostic was difficult to make, some further studies (other samples, different system sizes) were performed.

Finally the dashed lines adjacent to the pure case ( $\varepsilon = 0$ ) marking the limit of ergodicity (in panels (b) and (d) of Fig. 1 and Fig. S1 have been determined by visual inspection of the timeseries of  $\theta_m$ , the angle of the global polarity. In practice, 8 ordered initial conditions at regularly spaced angles are followed for  $10^6$  timesteps. The sample is declared ergodic if one of them displays a wandering global angle during the second half of the run. The location of this finite-size ergodicity limit does not depend much on this protocol.

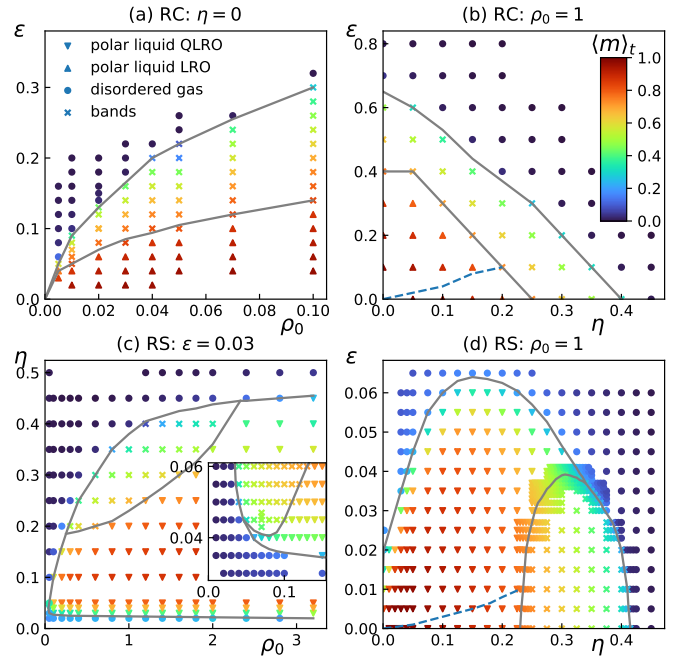

FIG. 1. Original data from which the stylized finite-size phase diagrams of Fig. 1 of the main text were drawn. At each run performed, a diamond colored by the estimated values of  $\langle m \rangle_t$  is represented. Top: RC case: (a)  $(\rho_0, \varepsilon)$  plane for  $\eta = 0$ ; (b)  $(\eta, \varepsilon)$  for  $\rho_0 = 1$ . Bottom: RS case: (c)  $(\rho_0, \eta)$  plane at fixed  $\varepsilon = 0.03$  (the inset shows the small- $\rho_0$ , small- $\eta$  region); (d)  $(\eta, \varepsilon)$  for  $\rho_0 = 1$ . The system size  $L = 256$  for all panels except in (a) and inset of (c), where  $L = 1024$  is used to delimit the band phase at small- $\rho_0$  and small- $\eta$  region.

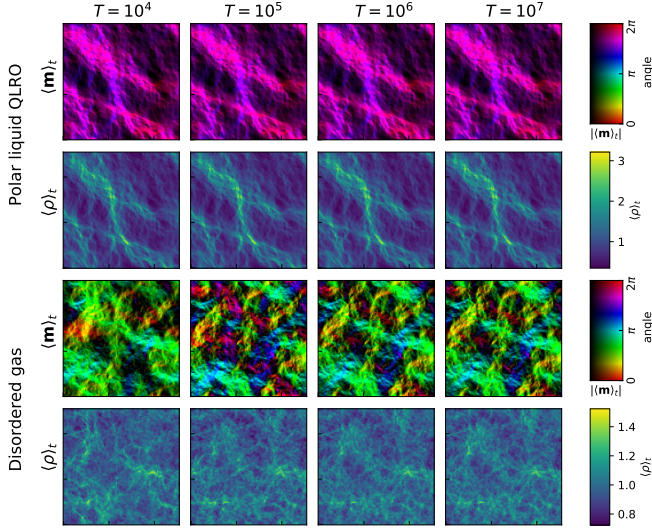

FIG. 2. Time-averaged momentum and density fields in RS case. Each image is averaged over  $T$  time steps, which increases from left to right.  $L = 512$ ,  $\eta = 0.18$ ,  $\epsilon = 0.035$  for the first two rows and 0.055 for the last two rows.

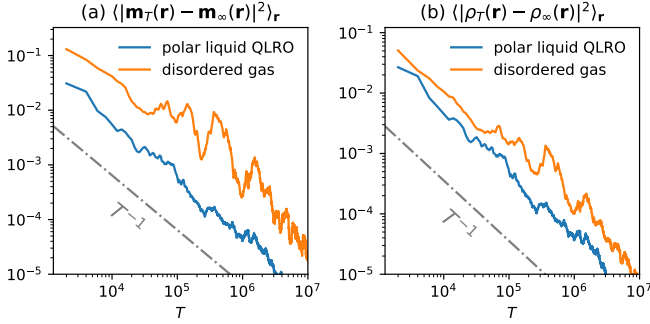

FIG. 3. (a)  $\langle |\mathbf{m}_T(\mathbf{r}) - \mathbf{m}_\infty(\mathbf{r})|^2 \rangle_{\mathbf{r}}$  and (b)  $\langle |\rho_T(\mathbf{r}) - \rho_\infty(\mathbf{r})|^2 \rangle_{\mathbf{r}}$  as function of  $T$  in RS case. Same parameters as in Fig. S2.

### Convergence of long-time average of coarse-grained fields

To construct the long-time averaged fields presented in the main text, we first build instantaneous coarse-grained fields, using the unit boxes over which quenched disorder is defined. (Using a larger elementary coarse-graining scale does not influence much the results.). Thus, the

density field  $\rho(\mathbf{r}, t)$  just counts the number of particles present in each box at time  $t$ . Likewise, the momentum field  $\mathbf{m}(\mathbf{r}, t)$  simply consists in the sum of the unit vectors  $\mathbf{e}_i^t$  over the particles  $i$  present in each box.

All long-time averaged momentum fields  $\mathbf{m}_\infty(\mathbf{r})$  presented in the main text are asymptotic: we checked that several of them calculated from different but long-enough timeseries are essentially identical, as shown in Fig. S2. In Fig. S3, we show that  $\langle |\mathbf{m}_T(\mathbf{r}) - \mathbf{m}_\infty(\mathbf{r})|^2 \rangle_{\mathbf{r}}$  and  $\langle |\rho_T(\mathbf{r}) - \rho_\infty(\mathbf{r})|^2 \rangle_{\mathbf{r}}$ , which quantify the difference between images averaged over  $T$  and the longest-average image, decay with  $T$  and become vanishing at large  $T$ .

### Attractor statistics

To obtain the attractor statistics shown in Fig. 2(g,h) of the main text, at each system size studied, we usually generate 500 samples in RS case and 350 samples in RC case. For each sample we run 8 simulations starting with ordered initial conditions, with initial  $\theta_m = 0, \pi/4, \pi/2, 3\pi/4, \pi, 5\pi/4, 3\pi/2, 7\pi/4$  respectively. Each run up is  $2E6$  time steps and we regard the resulting timeseries of  $\theta_m$  as steady if  $\theta_m$  stays around a preferred angle in the last  $1E6$  timesteps. A sample is classified 'steady' if all 8 timeseries for this sample are steady. In this case, we can further count the number of attractors for this sample, which can be easily read out from a polar plot of  $\theta_m$  similar to that of Fig. 2(a, b). After tagging each sample as non-steady or 1-, 2-, 3-, 4-attractor one, we finally obtain the fraction of each state shown in Fig. 2(g,h).

### Measuring $\chi_{att}$ , $\chi_{dis}$ , and $\chi_{tot}$ in RS case

Here we give some details about how the various RS-case susceptibilities presented in Fig. 4 and 5 of the main text have been calculated in practice.

Since samples exhibiting two attractors are dominant for the range of system sizes studied, as shown in Fig. 2(h) of the main text, we restricted ourselves to those, calculating  $\chi_{att}$  from the difference of  $\langle m \rangle_t$  between the 2 attractors of each sample.

Moreover, since the attractor fluctuations are typically much smaller than sample-to-sample fluctuations, we calculated  $\chi_{dis}$  from many samples for which we only ran a single initial condition.
